# Supplementary material for: Leveraging Transformer-based Language Models to Automate Requirements Satisfaction Assessment
Source: arXiv:2312.04463 source file (2023-12-07)
Supplement: Supplementary file 1 [file 07-Appendix.tex]

\section*{Appendix}
%-----------------------------Baselines--------------------------------
\ap{Fix it later}
Appendix Anonymous Link:
% https://docs.google.com/spreadsheets/d/e/2PACX-1vQEjPubJzx3T7U4LGOHCXhGPrbxiNEWXPCGXtLvzJie7ExIx3LVxc8-digz1d20tXclvXIJ6BvulAPv/pubhtml?gid=821469945&single=true

\href{https://docs.google.com/spreadsheets/d/e/2PACX-1vQEjPubJzx3T7U4LGOHCXhGPrbxiNEWXPCGXtLvzJie7ExIx3LVxc8-digz1d20tXclvXIJ6BvulAPv/pubhtml?gid=821469945&single=true}{Appendix}

\begin{itemize}
    \item A1: Baseline for C1 and C3! 
    \item A2: Baseline for C2
    \item A3: ML results for C2 based on the design length as we only report the requirement with 4 design elements in the paper. This table has results from  vanilla BERT, multitasking BERT, and dual BERT!
\end{itemize}

%Baselines for C1, C2 and C3 challenges
% \input{tables/BaselinesC1&C3}
% \input{tables/BaselineC2}

% Results of all challenges using LMs -- ths includes DMSat version as well though we do not use it in comparison or in any of the RQs?? Should we keep it 
% \input{tables/ChallengeC1}

% \input{tables/ChallengeC2}
% \input{tables/ChallengeC2Dual}

% \input{tables/ChallengeC3}
